# Supplementary material for: Sign of hard X-ray pulsation from the gamma-ray binary system LS 5039
Source: arXiv:2009.02075 source file (2020-09-04)
Supplement: Supplementary file 1 [file PRL_LS5039_suppl_5th_fin.pdf]

# Supplemental Material:
# Sign of hard X-ray pulsation from the gamma-ray binary system LS 5039

H. Yoneda,[1,2,3] K. Makishima,[2,1] T. Enoto,[4] D. Khangulyan,[5] T. Matsumoto,[1] and T. Takahashi[2,1]

[1] *Department of Physics, The University of Tokyo, 7-3-1 Hongo, Bunkyo, Tokyo 113-0033, Japan*
[2] *Kavli Institute for the Physics and Mathematics of the Universe (WPI), University of Tokyo, Kashiwa, Chiba 277-8583, Japan*
[3] *RIKEN Nishina Center, 2-1 Hirosawa, Wako, Saitama 351-0198, Japan*
[4] *Extreme natural phenomena RIKEN Hakubi Research Team, Cluster for Pioneering Research, RIKEN, Hirosawa 2-1, Wako, Saitama, 351-0198, Japan*
[5] *Department of Physics, Rikkyo University, 3-34-1 Nishi Ikebukuro, Toshima, Tokyo 171-8501, Japan*

## A. PULSE SEARCHES WITHOUT ORBITAL-MOTION CORRECTIONS

### A1. The system parameters of LS 5039

A binary system with the known orbital period $P_{\rm orb}$, like LS 5039, has four unknown parameters (except the orbital eccentricity); the primary star's mass $M_{\rm pr}$, the compact-object mass $M_{\rm x}$, the binary separation $a$, and the system inclination $\theta$. Optical spectroscopy can directly constrain $M_{\rm pr}$, and provide the orbital Doppler velocity amplitude $K$ of the primary. The third information is provided by X-ray pulse studies, like the present one, which can constrain $a_{\rm x} \sin\theta$, where $a_{\rm x} \equiv a\, M_{\rm pr}/(M_{\rm pr} + M_{\rm x})$. Then, the simple two-body Newtonian dynamics gives

$$\frac{M_{\rm x}}{M_{\rm pr}} = \frac{K}{a_{\rm x} \sin\theta} \left(\frac{P_{\rm orb}}{2\pi}\right) . \quad (1)$$

When combined with the optical information on $M_{\rm pr}$ and $K$ of LS 5039 from Ref.[1], Eq.(1) gives a fiducial relation describing LS 5039; the typical neutron-star mass of $M_{\rm x} = 1.4 M_\odot$ translates to $a_{\rm x} \sin\theta = 56^{+6}_{-8}$ light-sec. Further considering errors associated with Eq.(1), a mass estimate of $M_{\rm x} = (1.23 - 2.35)\ M_\odot$ has been derived as described in the main text. Similarly, this fiducial orbital radius of LS 5039 in turn predicts the orbital velocity of the neutron star to be $\sim 10^{-3}c$ as discussed in the main text.

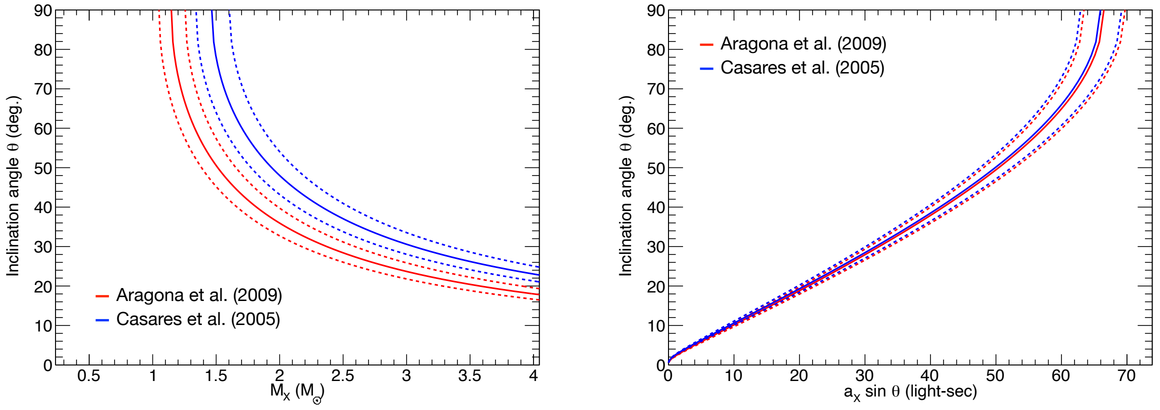


FIG. 1. The constraint of Eq.(2) for LS 5039, expressed on the $\theta$ vs. $M_{\rm x}$ (left) and $\theta$ vs. $a_{\rm x} \sin\theta$ (right) planes. The blue/red lines are based on the parameters from [1] and [2] respectively. The dotted lines indicate 1-sigma confidence intervals.

The last piece of constraint in the orbital-parameter determination is provided by the Kepler's third law, which relates a combination of the unknowns to that of the observables, as

$$\frac{(M_{\rm x} \sin\theta)^3}{(M_{\rm pr} + M_{\rm x})^2} = \frac{P_{\rm orb} K^3}{2\pi G} \sim 0.0026\ M_\odot \quad (2)$$

where $G$ is the constant of gravity, and the numerical value refers to the case of LS 5039 [2]. This quantity is often called the mass function. Figure 1 depicts this constraint for LS 5039, in two forms which are equivalent from Eq.(1).

### A2. Some remarks on Eq.(2) of the main text

Equation (2) of the main text may need some explanation, because the search range of $P_{\rm NS} > 1$ s we have selected and our choice of $\Delta T$ (4096, 8192, and 16384 sec) are somewhat inconsistent with Eq. (2). First, the search condition of $P_{\rm NS} > 1$ s was set based on the following consideration. The 10–30 keV source photon count rate with the *Suzaku* HXD is 81522 (photons)/500 (ks) $\times$ 10% $\simeq 1.6 \times 10^{-2}$ photons/s. If requiring $\Delta T = P_{\rm NS}/(1 \times 10^{-3}) = 1 \times 10^{3} P_{\rm NS}$, the number of source photons in each subset becomes $\sim 16 \times (P_{\rm NS}/1$ s). Since we need at least $\sim 10$ source photons to perform the Fourier transform, we have limited our pulsation search to $P_{\rm NS} > 1$ s. (This means that our approach of dividing the data becomes less effective for shorter pulse periods.) Then, Eq.(2) of the main text indicates that we should select $T = 1024$ sec and longer. However, the cases with $\Delta T = 1024$ and 2048 sec in practice interfere with the data gaps of similar lengths, which are caused by the *Suzaku*'s revolution around the Earth with a period of about 5.6 ks. To avoid this technical problem, we did not use $\Delta T = 1024$ or 2048 sec. This would not affect our approach, because the requirement of Eq. (2) is only approximate, with a tolerance by a factor of a few.

### A3. Demonstration of the pulse search by dividing data

In Figure 2, we demonstrate how the data division works in the Fourier analysis. We simulated the pulsation data with a pulse period of 5 s, assuming $P_{\rm orb} = 3.90608$ days, $a_{\rm x} \sin\theta = 50.0$ light-sec, $e = 0.30$, $\omega = 56$ deg., $\tau_0 = 0.0$, and the same photon counts and exposure time as the actual *Suzaku* HXD data. Then, the Fourier power spectra with/without the data division were produced. For reference, the power spectra simulated without invoking the binary motion are also presented. When we Fourier transform the entire data at once without dividing them into subsets, the power spectrum obviously has a good time resolution as in the left panel, but the Fourier peak becomes almost completely smeared out when the binary motion sets in. On the other hand, when we divide the data into subsets with $\Delta T = 4192$ sec (right panel), the Fourier analysis becomes much less affected by the binary motion at the expense of the time resolution.

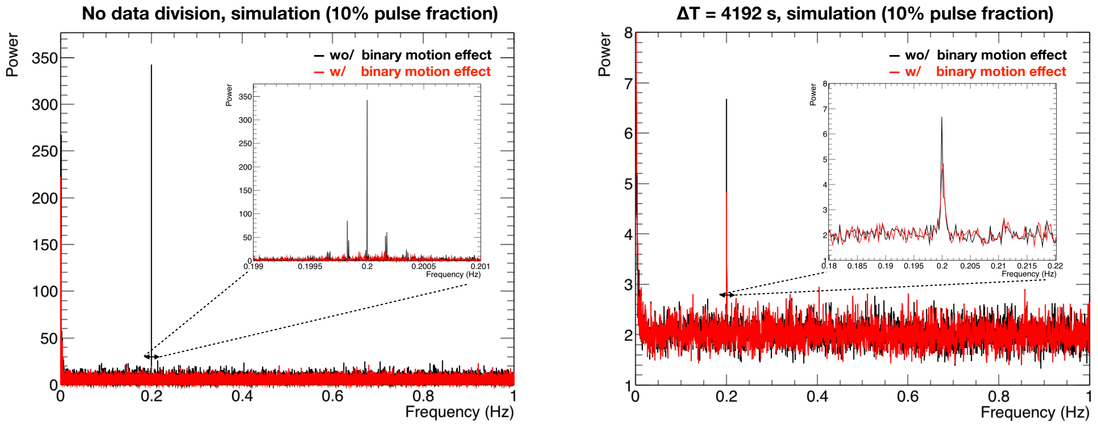


FIG. 2. Advantages of dividing data into subsets in Fourier analysis of the pulsar data. The left and right figures are the results without and with dividing the data respectively. The black and red lines indicate the results without and with the orbital motion, respectively.

## B. CONFIRMATION OF THE PURE POISSON NOISE IN THE FOURIER POWER SPECTRUM

When we calculate the significance of the Fourier peak in the *Suzaku* power spectrum, it is assumed that each power obeys the $\chi^2$ distribution. This assumption is valid only when the power spectrum is dominated by Poisson noise. Thus, in order to confirm that there are no other noise components, *e.g.* red noise, we performed the following four supplemental analyses.

We first investigated the distribution of the powers in the Fourier power spectrum. The left panel of Figure 3 shows the histogram of powers, derived from the 55 power spectra of the divided *Suzaku* data ($\Delta T = 8192$ s). We compared it with a chi-square distribution with 2 dof ($\propto \exp(-0.5x)$). The normalization of the chi-square distribution was fixed to the value expected from the number of the individual Fourier components and the pure Poisson noise. The

histogram is well described by the chi-square distribution, because the chi-square value of the comparison was $\chi^2$/dof = 39.4/31. Thus, the power distribution is consistent with the chi-square distribution with 2 dof. In Figure 1 (a) in the main text, the power spectrum was obtained by averaging all the power spectra from individual subsets. When $\Delta T = 8192$ s, the number of the subsets was 55. Therefore, each power in the averaged power spectrum should obey a chi-square distribution with 110 (= $2 \times 55$) dof.

As a second check, we rebinned the *Suzaku* power spectrum which was derived with $\Delta T = 8192$ s, and fitted it with a single powerlaw from 0.01 Hz to 1 Hz. The free parameters in the fitting were the normalization and the powerlaw index. The right panel of Figure 3 shows the result. The powerlaw index was obtained as $(-0.6 \pm 2.4) \times 10^{-3}$, which is consistent with an absence of any frequency-dependent noise component. Hence, this result gives another evidence that the power spectrum is dominated by Poisson noise.

The Fourier power spectrum has several peaks below 0.001 Hz. These are thought to arise from data gaps in the satellite data, caused by Earth occultations and the South Atlantic Anomaly. However, these Fourier components do not contribute at all to the power spectrum above $\sim$ 0.002 Hz.

Finally, we examined whether the $Z^2$ (m=4) values from the *Suzaku* and *NuSTAR* data obey the chi-square distribution of 8 dof, which was assumed in the orbital parameter searches. In this case, the period search range was very narrow, and the $Z^2$ (m=4) values derived from adjacent periods are correlated with each other. Thus, by broadening the period range, we employed the following steps. We sampled a period randomly from 0.01 s to 100 s, and calculated the $Z^2$ (m=4) value for that. By repeating this process, we obtained a distribution of the $Z^2$ (m=4) values, and compared it with the chi-square distribution in Figure 4. Again the normalization of the chi-square distribution was fixed to the expected value. This comparison yielded $\chi^2$/dof = 53.1/47 and 72.6/47 for *Suzaku* and *NuSTAR* respectively. Thus, the obtained distributions are adequately described with the chi-square distribution of 8 dof.

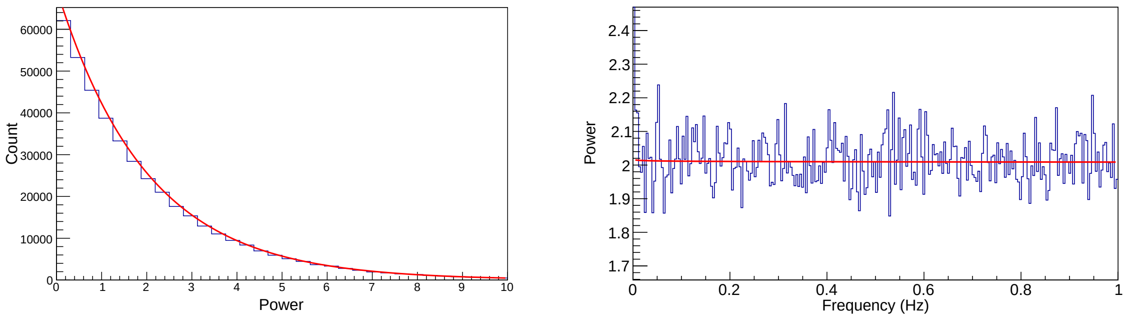


FIG. 3. The confirmation of the pure Poison noise in the power spectrum. (Left) The power distribution of the *Suzaku* Fourier power spectrum. (Right) The re-binned *Suzaku* power spectrum, fitted with a power-law function.

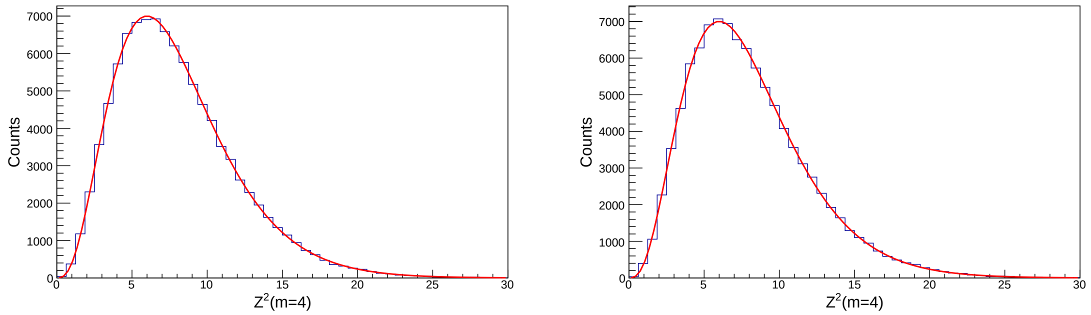


FIG. 4. The distribution of $Z^2$ (m=4) values sampled from the 0.01–100 s period range. The left and right panels show the *Suzaku* and *NuSTAR* data, respectively. The red lines represent the theoretically predicted chi-square distributions of 8 dof, with their normalizations fixed to the theoretically predicted value.

## C. POSSIBILITY OF CONTAMINATION FROM UNRELATED X-RAY SOURCES

Since the HXD of *Suzaku* is a non-imaging collimated detector and has a relatively large field-of-view of $34' \times 34'$ at energies below 100 keV, the detected pulsed emission could have originated from some unrelated sources near LS 5039. Among cataloged celestial objects, the one nearest to LS 5039 is NVSS J182535−1455555, separated from LS 5039 by $\sim$ 11 arcmin [3]. It is a radio source detected at 4.8 GHz [4], but is not cataloged as an X-ray emitter. Thus, it is unlikely to be a contamination source. Also, an isolated radio pulsar PSR J1825−1446 and a Wolf-Rayet star WR 115 (CXOU J182531.4−1444036) are at the edge of the HXD field-of-view. The spin period of PSR J1825−1446 is reported to be 0.28 s [5]. As for WR 115, *Chandra* observations detected 780 s periodic signals and a hint of 5000 s periodicity [6]. However, neither of the objects is reported to have a periodicity at $\sim$ 9 s. Therefore, we conclude that the pulsed signal detected with the HXD is not due to contamination from nearby sources. This conclusion is also supported by the *NuSTAR* confirmation of the (presumably) same periodicity, in which the utilized data accumulation region of 30 arcsec in radius is much smaller than that of the HXD and hence excludes all the candidates above.

## D. CONSISTENCY BETWEEN THE FOURIER AND Z$^2$ ANALYSES OF THE *NUSTAR* DATA

From the *NuSTAR* data, our Fourier analysis failed to find a significant periodicity, whereas a hint of 9.046 s period was obtained with the Z$^2$ analysis. This apparent discrepancy can be explained in terms of the different period/frequency ranges employed by the two methods. In the Z$^2$ analysis, the period search range was limited to 7 s to 11 s. This corresponds to 0.09–0.14 Hz in the frequency space, and is about 20 times narrower than that used in the Fourier analysis (1–100 Hz). Then, when the chance probability is $3.5 \times 10^{-3}$ in the limited 7–11 s range, that in the wider 1–100 Hz range would become 0.07 ($= 3.5 \times 10^{-3} \times 20$), which is consistent with the Fourier non-detection.

## E. CORRECTIONS FOR THE ORBITAL MOTION

In order to confirm the $8.960 \pm 0.009$ s and $9.046 \pm 0.009$ s periodicities found with the *Suzaku* and *NuSTAR* data, respectively, we applied the orbital correction to the two data sets. Referring to the orbital solutions reported in previous optical observations [1, 2, 7], we defined the search ranges of the four orbital parameters, and that of the pulse period, as described in Table I of the main text. The parameter search was then executed in the following manner: (1) An orbital parameter set is chosen from the defined parameter space. (2) The arrival times of individual photons are corrected for the orbital motion that is implied by the selected set of parameters. (3) By scanning the pulse period over the range defined in Table I of the main text, we register the maximum value ($\mathrm{Z}^2_{\mathrm{MAX}}$) of the Z$^2$ statistics from the corrected data. Here, up to the 4th harmonics are summed up. (4) By scanning the four orbital parameters over the respective ranges, we search for the parameter set that maximizes the $\mathrm{Z}^2_{\mathrm{MAX}}$ value.

Figure 5 shows the results of the orbital correction. The color contour indicates the maximum Z$^2$ value at each point on the ($a_{\mathrm{x}} \sin\theta,\ e$) plane when the other 3 parameters are all allowed to vary. The left panel is the *Suzaku* result, where a clear peak, indicated as (A), is seen around $(a_{\mathrm{x}} \sin\theta, e) \sim (53\ \text{light-sec}, 0.28)$. It corresponds to the orbital solution in Table I of the main text. It gives $\mathrm{Z}^2_{\mathrm{MAX}} = 67.28$ [8], which is 14.8 standard deviations above the mean of 8.0 when referring to a chi-square distribution of 8 (twice the maximum harmonic) dof. As described in the main text L.201, this gives the pre-trial probability of $1.7 \times 10^{-11}$.

The right panel of Figure 5 is the *NuSTAR* result. In this case, several peaks were found: one is around $(a_{\mathrm{x}} \sin\theta, e) \sim (48\ \text{light-sec}, 0.30)$ as indicated as (B), and several peaks are seen around $a_{\mathrm{x}} \sin\theta \sim 62 - 63$ light-sec as indicated as (C). These solutions have comparable significance, with $\mathrm{Z}^2_{\mathrm{MAX}} \approx 67$, to that of (B). However, as can be seen in Figure 1 (right), the latter solutions imply the system inclination of $\theta \sim 70^\circ \pm 6^\circ$, which is somewhat inconsistent with the constraint of $\theta < 66^\circ \pm 2^\circ$ [9] set by the lack of X-ray eclipses. In addition , (B) is closer to (A), though still somewhat inconsistent with each other. We hence consider that the solutions (C) are less likely than (B), and have adopted (B) in Table I in the main text.

## F. PULSE PROPERTIES IN DIFFERENT EPOCHS

The orbital solutions obtained from the two data sets have several issues (see the main text for the detail), including in particular the *Suzaku* vs. *NuSTAR* discrepancy on $a_{\mathrm{X}} \sin\theta$ and $e$. To obtain clues to these issues, we investigated how the pulse properties evolved through each observation. We divided the data into several subsets with similar time

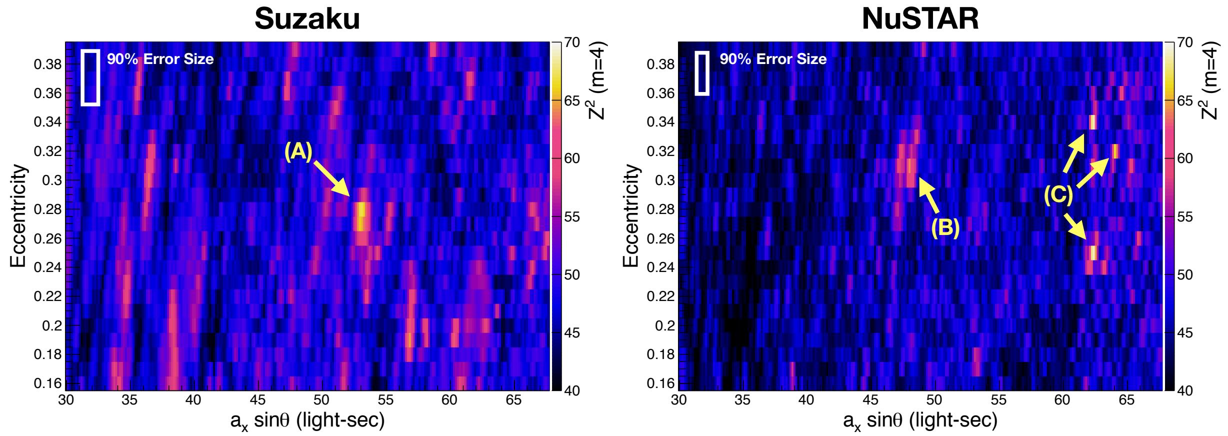


FIG. 5. $Z^2$ statistics considering the orbital motion of LS 5039. The colors indicate the $Z^2_{\rm MAX}$ values after the orbital correction, shown on a plane of the projected orbital radius of the compact star ($a_{\rm x}\sin\theta$, abscissa) and the orbital eccentricity ($e$, ordinate). The left and right figures are obtained using the 10–30 keV *Suzaku* and *NuSTAR* data respectively.

lengths, and calculated a 10-bin pulse profile in each epoch. The photon arrival times of the two data were corrected assuming the orbital solutions in Table I of the main text. In order to secure more than 100 source photons in each bin of the pulse profiles, we set the number of subsets as 7 and 5 for the *Suzaku* and *NuSTAR* data respectively.

The results are shown in Figure 6, for *Suzaku* (left) and *NuSTAR* (right), respectively. In both cases, the pulsation is seen throughout the observation. However, the pulse-peak phase and/or the pulse profiles are seen to fluctuate from time to time. Especially, this effect is more significant in the *NuSTAR* data; the main peak of the time-averaged pulse profile (Figure 2 in the main text) is clearly seen in the 2nd and 4th epochs, whereas the other epochs are dominated by either of the two sub-peaks of the time-averaged pulse profile. These results indicate that the pulse profile and/or the pulse phase would change considerably on time scales of several tens ksec. Presumably, these systematic effects have enhanced the side lobes seen in Figure 5, and biased the two orbital solutions beyond the nominal statistical uncertainties. Furthermore, the larger profile variation in *NuSTAR* than in *Suzaku* might explain the lower pulse fraction with *NuSTAR*.

## G. NOTE ON THE PULSE SEARCH IN THE SOFT X-RAY BAND

In the main text, we reported the upper limit of the pulse fraction in the soft X-ray band using the *NuSTAR* data since it covers from 3 keV to 78 keV. On the other hand, the *Suzaku* HXD data which we analyzed in this work covers from 10 keV to 70 keV. Thus, we cannot perform the soft X-ray pulse search using this HXD data. *Suzaku* has a co-aligned soft X-ray instrument (the XIS). However, its time resolution is 8 seconds since the focal plane detectors are CCDs, and this poor time resolution hampered the pulse study. Therefore, the soft X-ray pulse search was perfomed with only the *NuSTAR* data.

## H. KINETIC ENERGY OF THE STELLAR WINDS

Even when the mass accretion is somehow hampered, some energy is still available when the stellar winds hit the pulsar's magnetosphere. Assuming that the primary star launches isotropic stellar winds with a velocity $w$ at a mass-loss rate $\dot{M}_{\rm w}$, the kinetic wind energy $L_{\rm w}$ given to the pulsar's magnetosphere is calculated as

$$L_{\rm w} \sim \frac{1}{2}\dot{M}_{\rm w}w^2 \times \frac{\pi R_{\rm A}^2}{4\pi a_{\rm x}^2} \quad (3)$$

$$= 0.6\times 10^{25} \times \left(\frac{\dot{M}_{\rm w}}{10^{-6}M_\odot\ {\rm yr}^{-1}}\right)\left(\frac{w}{2000\ {\rm km/s}}\right)^2\left(\frac{R_{\rm A}}{2\times 10^8\ {\rm m}}\right)^2\left(\frac{a_{\rm x}}{50\ {\rm light\ sec}}\right)^{-2}\ {\rm W} \quad (4)$$

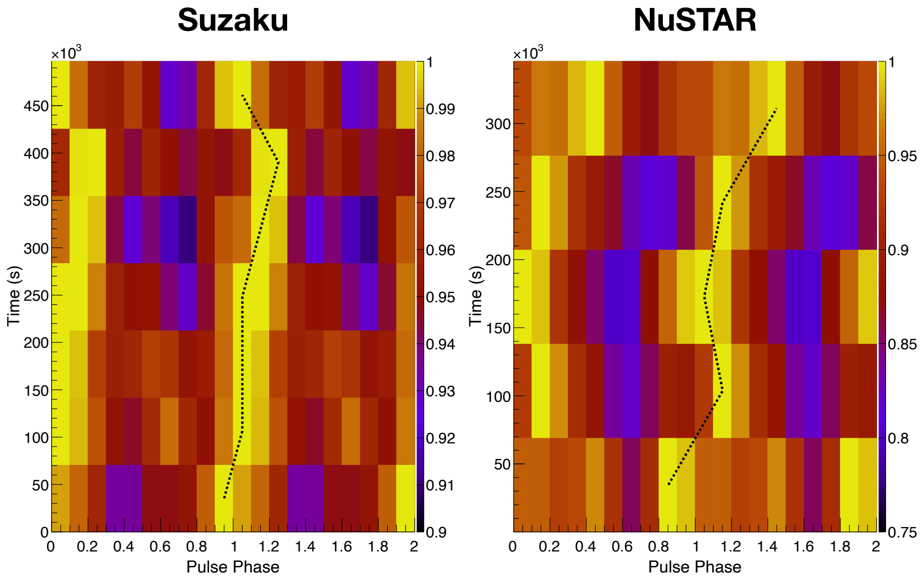


FIG. 6. Pulse profiles from *Suzaku* (left) and *NuSTAR* (right), derived in 7 and 5 time epochs, respectively. The orbital correction has been applied to the data, assuming the solutions in Table I of the main text. Each pulse profile was smoothed with a running average over three adjacent bins, and was normalized to its maximum bin value. The dashed lines indicate the pulse peak phases at different time epochs.

where $a_{\rm x}$ is the binary separation and $R_{\rm A}$ is the Alfvén radius (see the main text). Here, $10^{-6} M_{\odot}$ yr$^{-1}$ is the upper limit on the wind mass-loss rate from the primari star of LS 5039, reported in an optical observation [1]. This $L_{\rm w}$ is orders of magnitude too low to support the output of LS 5039.

[1] J. Casares, M. Ribo, I. Ribas, J. M. Paredes, J. Marti, and A. Herrero, A possible black hole in the gamma-ray microquasar LS 5039, Monthly Notices of the Royal Astronomical Society **364**, 899 (2005).

[2] C. Aragona, M. V. McSwain, E. D. Grundstrom, A. N. Marsh, R. M. Roettenbacher, K. M. Hessler, T. S. Boyajian, and P. S. Ray, The orbits of the gamma-ray binaries LS I +61 303 and LS 5039, Astrophys. J. **698**, 514 (2009).

[3] J. Moldón, M. Ribó, J. M. Paredes, W. Brisken, V. Dhawan, M. Kramer, A. G. Lyne, and B. W. Stappers, On the origin of LS 5039 and PSR J1825-1446, Astron. & Astrophys. **543**, A26 (2012).

[4] J. J. Condon, W. D. Cotton, E. W. Greisen, Q. F. Yin, R. A. Perley, G. B. Taylor, and J. J. Broderick, The NRAO VLA Sky Survey, The Astronomical Journal **115**, 1693 (1998).

[5] G. Hobbs, A. G. Lyne, M. Kramer, C. E. Martin, and C. Jordan, Long-term timing observations of 374 pulsars, Monthly Notices of the Royal Astronomical Society **353**, 1311 (2004).

[6] M. P. Muno, B. M. Gaensler, A. Nechita, J. M. Miller, and P. O. Slane, A Search for New Galactic Magnetars in Archival Chandra and XMM-Newton Observations, Astrophys. J. **680**, 639 (2008).

[7] G. E. Sarty, T. Szalai, L. L. Kiss, J. M. Matthews, K. Wu, R. Kuschnig, D. B. Guenther, A. F. J. Moffat, S. M. Rucinski, D. Sasselov, W. W. Weiss, R. Huziak, H. M. Johnston, A. Phillips, and M. C. B. Ashley, The $\gamma$-ray binary LS 5039: mass and orbit constraints from MOST observations, Monthly Notices of the Royal Astronomical Society **411**, 1293 (2011).

[8] Note that this value is slightly different from the $Z^2$ value described in Table I of the main text. This is because the value in the main text was obtained after finer search steps were employed around this peak, as described in the main text L.183.

[9] P. Reig, M. Ribó, J. M. Paredes, and J. Martí, Long-term X-ray variability of the microquasar system LS 5039/RX J1826.2-1450, Astron. & Astrophys. **405**, 285 (2003).
